# Supplementary material for: Using posterior predictive distributions to analyse epidemic models: COVID-19 in Mexico City
Source: arXiv:2005.02294 ancillary file (2020-05-15)
Supplement: Supplementary file 1 [file SIFinal.pdf]

# Supplementary Information for

## Using posterior predictive distributions to analyse epidemic models: COVID-19 in Mexico City

**Ramsés H. Mena, Jorge X. Velasco-Hernandez, Natalia B. Mantilla-Beniers, Gabriel A. Carranco-Sapiéns, Luis Benet, Denis Boyer and Isaac Pérez Castillo**

**isaacpc@fisica.unam.mx**

**This PDF file includes:**

Supplementary text
Tables S1 to S2
SI References

## Supporting Information Text

We explain the calibration method used in the main text and how we estimate the posterior distributions.

## Estimation of the parameters' posterior distribution

To construct the parameter's posterior distribution $P(\boldsymbol{\theta}|\mathcal{D})$, we first need to discuss the choice of model likelihood $P(\mathcal{D}|\boldsymbol{\theta})$ and the prior distribution $P_0(\boldsymbol{\theta})$. Taking into account a possibly rather large value $N$ of the host population, and since it is not possible to have the empirical correlation matrix for the observational data, we take the model's likelihood to be:

$$P(\mathcal{D}|\boldsymbol{\theta}) = \frac{1}{\sqrt{(2\pi)^{rt_{\max}}}} \exp\left[-\frac{1}{2}\sum_{t=0}^{t_{\max}}\sum_{a=1}^{r}\left(\mathcal{N}_a(t,\boldsymbol{\theta}) - \mathcal{N}_a^{(\text{obs})}(t)\right)^2\right] , \qquad [1]$$

where we have assumed that the observational dataset is independent, that Gaussian variables are identically distributed, with unit variance, and $t_{\max}$ is the time of the last recorded data. Granted, this is a gross over-simplification as, in principle, these data are time and compartment correlated and one would need the corresponding empirical correlation matrix, for which we have no information.

Regarding the choice of $P_0(\boldsymbol{\theta})$, it would seem appropriate in principle to consider an empirical a priori distribution by gathering the resulting parameter values $\boldsymbol{\theta}$ obtained in studies from other countries. While this approach is indeed tempting from a statistical point of view, it assumes that health conditions, comorbidities and other important aspects are homogeneous among different countries, which is clearly untrue. Thus a cautious approach, aiming to avoid confirmation bias, is to use a flat prior within a range of parameters $\theta_a \in [\theta_a^{(\min)}, \theta_a^{(\max)}]$, where the boundaries of the parameters are reasonably wide, enough to be compatible with the available data from other studies. That is

$$P_0(\boldsymbol{\theta}) = \frac{1}{Z_0}\prod_{a=1}^{r}\mathbb{I}\left\{\theta_a \in [\theta_a^{(\min)}, \theta_a^{(\max)}]\right\} , \qquad [2]$$

where $Z_0$ is a normalization constant of the prior distribution and $\mathbb{I}$ is an indicator function. Given that the explicit solution of the evolution equations of the model is not always available, the resulting parameter's posterior distribution $P(\boldsymbol{\theta}|\mathcal{D})$ is a rather complicated function of $\boldsymbol{\theta}$, so that the natural way to carry out the integrals appearing in the expressions of the predictive posteriors is by numerically estimating $P(\boldsymbol{\theta}|\mathcal{D})$ by a Monte Carlo method.

Before embarking the difficult task of calibrating the model using open data of SARS-CoV-2 cases in Mexico City, we sought to develop some intuition of the model's behaviour presented in the main text. Consequently, we addressed how the calibration behaves depending on the time window considered for the observational data. For an arbitrary, yet realistic, choice of the parameters, we generate a synthetic data set $\{\boldsymbol{N}^{(\text{syn})}(t)\}_{t=0}^{t_{\max}}$ and explore the MAP problem in terms of $t_{\max}$. We observed that for $t_{\max} < t_{\text{peak}}$ the posterior distribution is indeed rather flat while for $t_{\max} > t_{\text{peak}}$, a more defined maximum appears and the model is more easily calibrated. We must emphasize that these observations are neither new nor remarkable properties for this type of models. However, it emphasises that whichever analysis is performed on these models, particularly if they are intended as a forecasting tool, using data from the beginning of the epidemic curve alone renders great variability of possible outcomes and must be carried out reckoning these properties.

Thus, as we have observation data only at the beginning of the epidemic curve, and since we are dealing here with sloppy models, the parameter's posterior distribution is rather flat in most of the directions of the parameter space. This indicates that the most efficient approach is first to solve the minimization problem

$$\boldsymbol{\theta}^{\star} = \text{argmax}_{\boldsymbol{\theta}\in[\boldsymbol{\theta}^{(\min)},\boldsymbol{\theta}^{(\max)}]} P(\mathcal{D}|\boldsymbol{\theta}) , \qquad [3]$$

and then to explore uniformly the space of parameters around the point $\boldsymbol{\theta}^{\star}$, by randomly perturbing it with a random variable $\boldsymbol{\epsilon}$, that is $\boldsymbol{\theta}^{\star} \to \boldsymbol{\theta} = \boldsymbol{\theta}^{\star} + \eta\boldsymbol{\epsilon}$, with $\eta$ controlling the spread of the exploration in the parameter space. In this way, the two posterior predictive distributions presented in the main text are approximated by

$$\begin{aligned} P(\boldsymbol{n}, t|\mathcal{D}) &= \frac{1}{V_{\Omega_\eta(\boldsymbol{\theta}^\star)}}\int_{\Omega_\eta(\boldsymbol{\theta}^\star)} d\boldsymbol{\theta} P[\boldsymbol{\mathcal{N}}(t,\boldsymbol{\theta}) = \boldsymbol{n} \mid \boldsymbol{\theta}] , \\ P\left(\boldsymbol{t}_{\text{peak}}\middle|\mathcal{D}\right) &= \frac{1}{V_{\Omega_\eta(\boldsymbol{\theta}^\star)}}\int_{\Omega_\eta(\boldsymbol{\theta}^\star)} d\boldsymbol{\theta}\delta\left[\boldsymbol{t}_{\text{peak}} - \text{argmax}_t \boldsymbol{\mathcal{N}}(t,\boldsymbol{\theta})\right] , \end{aligned} \qquad [4]$$

which can be easily estimated by direct Monte Carlo sampling. Here $V_{\Omega_\eta(\boldsymbol{\theta}^\star)} = \int_{\Omega_\eta(\boldsymbol{\theta}^\star)} d\boldsymbol{\theta}$, and $\Omega_\eta(\boldsymbol{\theta}^\star)$ stands for the integration region in the parameter space, centered at $\boldsymbol{\theta}^\star$ and of width $\eta$. Throughout the whole text we have taken $\eta = 0.1$.

**Table S1. In this table we show some examples of estimated parameters from studies carried out in different countries**

| Parameter | Median | 95% credible interval or Range | Reference |
|---|---|---|---|
| Infection →onset of symptoms $\tau_l$ | 5.1 d | 4.5-5.8 d | (1) |
| Onset of symptoms → Death | 17.8 d | 16.9-19.2 d | (2) |
| Onset of symptoms → hospital discharge | 24.7 d | 22.9-28.1 d | (2) |
| Serial interval ($\approx \tau_i$) | 6.5 d | 5-8 (range) d | (3) |
| Prob. severe symptoms → ICU | 0.36 adults, 0.2 seniors | - | (4) |
| Hospitalized → R rate | 0.072 adults, 0.022 seniors (1/d) | - | (4) |
| Hospitalized → D rate | 0.0042 adults, 0.014 seniors (1/d) | - | (4) |
| ICU → R rate | 0.05 adults, 0.036 seniors (1/d) | - | (4) |
| ICU → D rate | 0.0074 adults, 0.029 seniors (1/d) | - | (4) |
| $R_0$ | 2.4 | 2-4.5 | (5) |

## Estimates from other countries

An important initial issue is how to define the prior distribution $P_0(\boldsymbol{\theta})$. For simplicity we consider a flat distribution in each of the parameters defining $\boldsymbol{\theta}$, whose ranges we base in estimates made in other countries; see Table S1.

In general, most countries have resorted in studies based on epidemic data from China, in order to understand and manage their outbreaks. Recent work (2) has reported that the mean duration from onset of symptoms to death is about 17.8 days (95% CI 16.9-19.2 days), and the mean duration from symptom onset to hospital discharge is 22.6 days (95% CI 21.1-24.4 days). The same paper has estimated the overall infection fatality rate for China to be 0.66% (0.39-1.33) with higher numbers for older ages. Also, they report that the percentage of individuals likely to be hospitalized increases with age to a maximum of 18.4% (11.0-7.6). Mizumoto *et al.* (6) report from their study of the Diamond Princess cruise ship, a proportion of asymptomatic cases of 17.9% (95% CI 15.5-20.2), with this estimate sensitive to the mean incubation period assumed. Nishiura *et al.* (7), using data from Wuhan, China, estimate the asymptomatic ratio (percentage of carriers with no symptoms) to be higher, at 30.8% (95% CI 7.7-53.8). Wang et al (8) report a varying average daily attack rate per million people for Wuhan depending upon on the evolution of the epidemic: 2.2 (95% CI 2.0-2.4) before January 11, 44.9 (43.6-46.2) between January 11 and January 22nd, 150.9 (148.3-153.5) between January 23rd and February 1st, and 54.1 (52.9-55.3) after February 2nd. However, differences in this rate were found depending on age and risk group (healthcare professionals). As for the severity of the disease, these authors report 49.9% mild, 27.4% moderate and 19.7% severe, although they point out that this last percentage decreased gradually to reach 14.7% in the last phase of the epidemic.

Health authorities in Mexico are apparently estimating the overall attack rate to be well below the highest attack rate reached in China (Jan 23rd-Feb 1st) of 150.9 per million people. However, the percentage of asymptomatic cases is in accordance with Nishiura *et al.* (7) estimate. The percentage of people requiring hospitalization is lower (9.8%) than the maximum of 18.4% reported (also for China) in (2).

## Calibration of model

When calibrating the model, we must note that the public dataset does not provide the total number of patients in each compartment. However, the number the new daily infected, hospitalized, critically-ill, is reported as well as the total number of deaths. Thus, when calibrating the model, the first three time series must be compared to the corresponding terms of the RHS of the equations. More precisely, the new daily infected cases is fitted to $E(t)/\tau_\ell$, the new daily hospitalized cases is fitted to $(1-m)\frac{I(t)}{\tau_i} + (1-f)\frac{C(t)}{\tau_c}$, the new daily critically-ill patients is fitted to $c\frac{H(t)}{\tau_h}$, and finally, the total number of deaths is fitted to $D(t)$.

All in all, given the dataset, we need to determine model parameters $\boldsymbol{\theta} = (\tau_i, \tau_\ell, \tau_h, \tau_c, m, c, f, R_0, \gamma)$, with initial conditions $(S(0), E(0) = I(0) \times \tau_\ell, I(0) = 5, H(0) = 1, C(0) = 1.5, R(0) = 0, D(0) = 0)$, where the initial time $t = 0$ is set to February 27th. Moreover, since we have no information on the initial conditions for $S(0)$, we will also consider this as a parameter to be fitted. For the contingency plan, we take $M(t)$ as step function representing the decrease in the effective contact rate induced by the mitigation measures (which has been smoothed for computational convenience) equal to 1 for $t$ smaller to 25 (corresponding to March 23rd, the data each which the mitigation plan was activated in Mexico) and equal to $\gamma$ for $t \geq 25$. The value of $N$ is obtained as $N = S(0) + E(0) + I(0) + H(0) + C(0) + R(0) + D(0)$, and each parameter is allowed to take values in the following range: $\tau_i \in [4, 9]$, $\tau_\ell \in [4, 6]$, $\tau_h, \tau_c \in [3, 15]$, $m, f \in [0.2, 0.8]$, $c \in [0.2, 0.7]$, $S(0) \in [0, 0.9N_{\text{pop}}]$, $R_0 \in [0.8, 5]$, and $\gamma \in [0, 1]$, where $N_{\text{pop}}$ is the population of Mexico City (around 9 million). These intervals have been chosen to be wide enough so that they are compatible with observations from other countries, trying to avoid any particular bias to a particular study.

We then proceed to maximize the parameters' posterior numerically according to Eq. [3]. The method is essentially a Monte Carlo one, integrating few million times the equations of motion with different parameters, and using a *black box* optimization method written in Julia (9), in order to maximise the likelihood. Table S2 shows the resulting optimal parameters $\boldsymbol{\theta}^\star$, including the initial susceptible and exposed population estimates, $S(0) = 54511$ and $E(0) = 16$, respectively.

**Table S2. Values of optimal parameters found by maximizing the parameter's posterior distribution.**

| Model's parameters | Interval range | Optimal parameters |
|---|---|---|
| $\tau_i$ | [4,9] | 5.49 days |
| $\tau_\ell$ | [4,6] | 4.98 days |
| $\tau_h$ | [3,15] | 3.0 days |
| $\tau_c$ | [3,15] | 3.0 days |
| $m$ | [0.2,0.8] | 0.6 |
| $c$ | [0.2,0.7] | 0.45 |
| $f$ | [0.2,0.8] | 0.8 |
| $R_0$ | [0.8,5] | 2.48 |
| $\gamma$ | [0,1] | 0.82 |

## References


1. SA Lauer, et al., The Incubation Period of Coronavirus Disease 2019 (COVID-19) From Publicly Reported Confirmed Cases: Estimation and Application. *Annals internal medicine* **2019** (2020).
2. R Verity, et al., Estimates of the severity of covid-19 disease. *MedRxiv* (2020).
3. NM Ferguson, et al., Impact of non-pharmaceutical interventions (NPIs) to reduce COVID- 19 mortality and healthcare demand. *Imp. Coll.* (2020).
4. L Di Domenico, G Pullano, CE Sabbatini, PY Boëlle, V Colizza, Expected impact of lockdown in île-de-france and possible exit strategies. *medRxiv* (2020).
5. S Flaxman, et al., Estimating the number of infections and the impact of non- pharmaceutical interventions on COVID-19 in 11 European countries, Technical Report March (2020).
6. K Mizumoto, K Kagaya, A Zarebski, G Chowell, Estimating the asymptomatic proportion of coronavirus disease 2019 (covid-19) cases on board the diamond princess cruise ship, yokohama, japan, 2020. *Eurosurveillance* **25** (2020).
7. H Nishiura, et al., The extent of transmission of novel coronavirus in wuhan, china, 2020. *J. Clin. Med.*, 330 (2020).
8. C Wang, et al., Evolving epidemiology and impact of non-pharmaceutical interventions on the outbreak of coronavirus disease 2019 in wuhan, china. *medRxiv* (2020).
9. R Feldt, A Stukalov, BlackBoxOptim.jl (https://github.com/robertfeldt/BlackBoxOptim.jl) (2018).
